# Supplementary material for: Solving Continual Combinatorial Selection via Deep Reinforcement Learning
Source: arXiv:1909.03638 source file (2019-09-09)
Supplement: Supplementary file 1 [file appendix.tex]

\onecolumn
% \section{Supplementary}
\begin{appendices}

\section{Intra-Parameter Sharings} \label{sec:IntraSharing}
\subsection{Intra-Parameter Sharing Layers} \label{sec:IntraSharing_math_single_channel}
In this section, we mathematically describe the intra-sharing layers $\phi_{k}^{A}$ and $\phi_{k}^{B}$ in Figure \ref{fig:eilayers}. 
Let $\mathbf{I}_k \in \mathbb{R}^{k \times k}$ an identity matrix and $\mathbf{1}_{k,k'} \in \mathbb{R}^{k \times k'}$ the matrix of ones. 
Let $\mathbf{I}_{x}:= \mathbf{I}_{\vert \bx_{k} \vert}$, $\mathbf{I}_{y}:= \mathbf{I}_{\vert \by_{k} \vert}$ and $\mathbf{1}_{x,y}:= \mathbf{1}_{\vert \bx_{k} \vert, \vert \by_{k} \vert}$ for simple notations which implicitly includes $k$ and $N$.

\noindent {\bf Layer $\phi_{k}^{A}$.} 
Let $\phi_{k}^{A}(\tbx_{k},\tby_{k}):=(\tbX_{k}, \tbY_{k})$ with $\tbx_{k}, \tbX_{k} \in \Real ^{k}$ and $ \tby_{k},  \tbY_{k} \in \Real ^{N-k}$ where  
\begin{align} \label{eq:phi_A_output_XY}
  \tbX:= \rho( \bw_{\tx}\tbx + \bw_{\tx \tx}\tbx +\bw_{\tx \ty}\tby + \bb_{\tx}), \qquad
  \tbY:= \rho( \bw_{\ty}\tby + \bw_{\ty \ty}\tby +\bw_{\ty \tx}\tbx + \bb_{\ty} )
\end{align} 
with a non-linear activation function $\rho$.
The parameter shared matrices $\bw_{x}, \cdots, \bw_{yy}$ defined as follows:
\begin{align*} 
  & \bw_{\tx}:=w_{\tx} \mathbf{I}_{x} ,\quad \bw_{\tx\tx}:=\frac{w_{\tx\tx}}{\vert \bx \vert} \mathbf{1}_{x,x} ,\quad \bw_{\tx\ty}:=\frac{w_{\tx\ty}}{\vert \by \vert} \mathbf{1}_{x, y}, \quad \bb_{\tx}:= b_{\tx} \mathbf{1}_{x, 1}, \\
  & \bw_{\ty}:=w_{\ty} \mathbf{I}_{y},\quad \bw_{\ty\ty}:=\frac{w_{\ty\ty}}{\vert \by \vert} \mathbf{1}_{y, y} ,\quad \bw_{\ty\tx}:=\frac{w_{\ty\tx}}{\vert \bx \vert} \mathbf{1}_{y, x}, \quad \bb_{\ty}:=b_{\ty} \mathbf{1}_{y, 1}. 
\end{align*}

The entries in the weight matrices $\bw_{\tx}, \cdots, \bb_{y}$ are tied by real-value parameters
$w_{\tx}, \cdots, b_{\ty} \in \Real$, respectively. 
Some weight matrices such as $\bw_{\tx\tx}, \bw_{\tx\ty}, \bw_{\ty\tx}, \bw_{\ty\ty}$ have normalizing term $\frac{1}{\vert \bx \vert}$ or $\frac{1}{\vert \by \vert}$.
These normalizations help inter-sharing between the different Q-Networks $Q_{k}$s with flexible dimensions as $k$ or $\vert \bx_{k} \vert$ varies.

\noindent {\bf Layer $\phi_{k}^{B}$.}
% The layer $\phi_{k}^{B}$ has similar architecture to $\phi_{k}^{A}$.
The difference of $\phi_{k}^{B}$ from $\phi_{k}^{A}$ is that the range of $\phi_{k}^{B}(\tbx, \tby)$ is restricted in $\tbY$ of \ref{eq:phi_A_output_XY}, i.e.,  $\phi_B(\tbx,\tby) :=\tbY \in \Real ^{N-k} $ where $ \tbY = \rho( \bw_{x}\tbx + \bw_{xx}\tbx +\bw_{xy}\tby  + \bb_{\ty}). $
The weight matrices are similarly defined as in the $\phi_{k}^{A}$ case:
\begin{align*} 
  \bw_{\ty}:=w_{\ty} \mathbf{I}_{y},\quad \bw_{\ty\ty}:= \frac{w_{\ty\ty}}{\vert \by \vert} \mathbf{1}_{y,y} ,\quad \bw_{\ty\tx}:=\frac{w_{\ty\tx}}{\vert \bx \vert} \mathbf{1}_{y,x}, \quad \bb_{\ty}:=b_{\ty} \mathbf{1}_{y, 1}. 
\end{align*}

\smallskip
\noindent {\bf Deep Neural Network with Stacked Layers.} The intra-sharing network $Q_{k}(\tbx, \tby)$ 
is generated by stacking $\phi^A_{k}$ multiple times including the input layer and setting the final layer by $\phi^B_{k}$, i.e., 
% which the composition of the layers $\phi_{k}^{A}$ and the final output layer is  $\phi_{k}^{B}$. 
\begin{align} \label{eq:einet}
  Q_{k}(\tbx, \tby) := (\phi^B_{k} \circ \phi^A_{k} \circ \cdots \circ \phi^A_{k}) (\tbx, \tby).
\end{align}
Under this definition, intra-sharing $Q_{k}(\tbx, \tby)$ always satisfies EI in \eqref{eq:equi-inv property}. 
\subsection{Multiple Channels}
\label{sec:multiplechannels}
\noindent {\bf Multiple Channels.} 
In the above section, we describe   simplified versions of the intra-sharing layers $$\phi_{k}^{A}: \Real^{\vert \bx \vert + \vert \by \vert} \rightarrow \Real^{\vert \bx \vert + \vert \by \vert}, \qquad \phi_{k}^{B}: \Real ^{\vert \bx \vert + \vert \by \vert}\rightarrow \Real ^{\vert \by \vert}.$$ 
In this section, we extend this to
\begin{equation} \label{eq:EILayers}
  \phi_{k}^{A}: \Real^{\vert \bx \vert \cdot P_{x} + \vert \by \vert \cdot P_{y}} \rightarrow \Real^{\vert \bx \vert \cdot O_{x} + \vert \by \vert \cdot O_{y}}, \qquad \phi_{k}^{B}: \Real^{\vert \bx \vert \cdot P_{x} + \vert \by \vert \cdot P_{y}} \rightarrow \Real^{\vert \by \vert \cdot O_{y}}
\end{equation}
where $P_{x}, P_{y}, O_{x}, O_{y}$ are the feature numbers of each item informations respectively. 
The role of the feature numbers is similar to that of channels in convolutional neural networks which increase the expressive power and handle the multiple feature vectors. 
% we can consider multiple input channels $P$ and output channels $O$.
This wider version of network with intra-sharing has more expressive power due to increased number of the hidden nodes, according to the \textit{universial approximatin theorem} \cite{gybenko1989approximation}. 
In here, we only handle the case for $P_{x} = P_{y} = P$ and $O_{x} = O_{y} = O$ for a concise description. 
We use superscripts $\bx^{\langle p \rangle}, \by^{\langle p \rangle} $ and $\bX^{\langle o \rangle}, \bY^{\langle o \rangle}$ to denote such channels. 
Our architecture satisfies that cross-channel interactions are fully connected. 
Layer $\phi_{k}^{A}(\tbx, \tby)$ with multiple channels is as follows:
\begin{align*}
  & \tbX^{\langle o \rangle}:= \rho\left( \sum_{p=1}^{P} \left(  \bw^{\langle o, p \rangle}_{\tx}\tbx^{\langle p \rangle} + \bw^{\langle o, p \rangle}_{\tx \tx}\tbx^{\langle p \rangle} +\bw^{\langle o, p \rangle}_{\tx \ty}\tby^{\langle p \rangle} + \bb^{\langle o \rangle}_{\tx} \right) \right), \\
  & \tbY^{\langle o \rangle}:= \rho\left(\sum_{p=1}^{P} \left( \bw^{\langle o, p \rangle}_{\ty}\tby^{\langle p \rangle} + \bw^{\langle o, p \rangle}_{\ty \ty}\tby^{\langle p \rangle} +\bw^{\langle o, p \rangle}_{\ty \tx}\tbx^{\langle p \rangle} + \bb^{\langle o \rangle}_{\ty} \right) \right)
\end{align*}
where 
\begin{equation} \label{eq:weight_multiple_channels}
  \begin{split}
  & \bw^{\langle o,p \rangle}_{\tx}:=w^{\langle o,p \rangle}_{\tx} \mathbf{I}_{x} ,\quad \bw^{\langle o,p \rangle}_{\tx\tx}:=\frac{w^{\langle o,p \rangle}_{\tx\tx}}{\vert \tbx \vert} \mathbf{1}_{x,x} ,\quad \bw^{\langle o,p \rangle}_{\tx\ty}:=\frac{w^{\langle o,p \rangle}_{\tx\ty}}{\vert \tby \vert} \mathbf{1}_{x,y}, \quad \bb^{\langle o \rangle}_{\tx}:= b^{\langle o \rangle}_{\tx} \mathbf{1}_{x, 1}, \\
 & \bw^{\langle o,p \rangle}_{\ty}:=w^{\langle o,p \rangle}_{\ty} \mathbf{I}_{\ty},\quad \bw^{\langle o,p \rangle}_{\ty\ty}:=\frac{w^{\langle o,p \rangle}_{\ty\ty}}{\vert \tby \vert} \mathbf{1}_{y, y} ,\quad \bw^{\langle o,p \rangle}_{\ty\tx}:=\frac{w^{\langle o,p \rangle}_{\ty \tx}}{\vert \tbx \vert} \mathbf{1}_{y,x}, \quad \bb^{\langle o \rangle}_{\ty}:=b^{\langle o \rangle}_{\ty} \mathbf{1}_{y, 1}.
  \end{split}
 \end{equation}
 Similar to the above cases, the entries in the weight matrices  $\bw^{\langle o,p \rangle}_{\tx}, \cdots, \bb^{\langle o \rangle}_{\ty}$ are tied together by real-value parameters $w^{\langle o,p \rangle}_{\tx}, \cdots, b^{\langle o \rangle}_{\ty}$ respectively. 
\smallskip

\section{Proofs}
\subsection{Theorem~\ref{thm:local optimal}}
\label{proof:local-optimal}
\begin{proof}
      
      To use contradiction, we first assume that there exists at least one local minima $\theta^{*} \in  \Theta$ in the loss function $l_{F}(s;\theta)$ 
      % which defined by the parameter shared neural network architecture $H_{\overline{\theta}}$ in the figure 
      while $ \overline{\theta}^{*} \in \ovT $ is not a local minima in the loss function $l_{G}(s;\ovt)$ in a network without parameter sharing $G(s;\ovt)$.
      Therefore, 
      there must be a vector $\Delta \ovt \in \ovT$ in the weight parameter space $\ovT$ which makes the directional derivative $D_{\Delta \ovt}(l_{G}(s;\overline{\theta}^{*}))$ negative. 
      % of the loss surface for $G_{\theta}$ along $\Delta \ovt$ from $\overline{\theta}^{*} \in \Theta$. In other words,  $ D_{\Delta \ovt}(G_{\overline{\theta}^{*}}) < 0.  $ 
    We first extend the definition of $\Sigma \in S_{M} \times S_{N}$ as the mapping $\Sigma:\ovT \rightarrow \ovT$.
    Under this extension, we can generate $M! \times N!$ more vectors $\Sigma(\Delta \ovt)$ for each $\Sigma$ that has the same directional derivatives compared to the derivative of $\Delta \ovt$, i.e. 
      \begin{equation} 
        \label{eq:DpiveqDv}
      D_{\Sigma(\Delta \ovt)} (l_{G}(s;\Sigma(\ovt^{*})))  = D_{\Delta \ovt} (l_{G}(s;\ovt^{*})).
      \end{equation}

\noindent{\textbf{The extended definitions for $ \Sigma=( \sigma, \sigma ')$}}

    %   Regard $\Sigma$ as a bijective mapping  $R^{N+M} \rightarrow R^{N+M}$, $R^{M} \rightarrow R^{M}$, and $\Theta \rightarrow \Theta$
       From now on, we will extend and abuse the original definition of $\Sigma$ in several but naturally inducible ways. 
       First of all, we extend $\Sigma$ as the permutation among both $\{1,2,...,M+N\}$ and $\{1,2,...,M\}$ where $\Sigma(i) = \sigma(i)$ when $i\leq M$ or $\Sigma(i)=M+\sigma'(i-M)$ when $i>M$.
       This extension just considers the case where  $\{1,2,...,M\}$ elements are selectable, $\{M+1,...,M+N\}$ elements are unselectable or only $M$ selectable elements exist, which are already reflected in EINET as $\phi_{k}^{A}$ for $\{1,2,...,M+N\}$ or $\phi_{k}^{B}$ for $\{1,2,...,M\}$.  
       For the second extension of $\Sigma$, it is the permutation among $\overline{\theta^{l}}$ which is the parameter set of  $l$th layer $\phi(s;\overline{\theta^{l}})$ in the deep neural network $G(s;\ovt)$.
       The $l$th layer $\phi(s;\overline{\theta^{l}}):\Real^{M+N} \rightarrow \Real^{M+N}$ or $\phi(s;\overline{\theta^{l}}):\Real^{M+N} \rightarrow \Real^{M}$ with   $\overline{\theta^{l}} = (\overline{\bw^{l}}, \overline{\bb^{l}} )$ is defined as  $\phi(s;\overline{\theta^{l}}) = \overline{\bw^{l}} s +\overline{\bb^{l}}$. 
       We define $\Sigma(\overline{\theta^{l}}) := (\Sigma(\overline{\bw^{l}}), \Sigma(\overline{\bb^{l}}))$, where 
       \begin{align} \label{eq:extensionwb}
       \Sigma(\overline{\bw^{l}})(\Sigma(j), \Sigma(i)) = \overline{\bw^{l}}(j,i) \quad \text{and} \quad \Sigma(\overline{\bb^{l}})(\Sigma(i)) = \overline{\bb^{l}}(i).
       \end{align}
       The weight parameters $\ovt $ for the deep neural network $G$ is just the collection of the weight parameters of each layers such as $\overline{\theta^{l}}$. 
       We can finally extend our final definition of $\Sigma$ as the permutations among $\ovt$.

    %    \note{HS:
    %    We first extend the definition of the mapping $\Sigma$  to the bijective mapping between nodes in $H_{\overline{\theta}}$ and then extend it to bijective mapping between the weight parameter space $\Theta$. 
    % %    For the input layer or the first hidden layer, there are $N$ invariant nodes and $M$  
    %    Each layer has $N$ invariant nodes  and  $M$ equivariant  nodes or  only $M $ equivariant nodes. 
    %    The mapping $\Sigma = (\sigma ', \sigma) $ maps $i$th invariant node to $\sigma '(i)$th invariant node as well as it maps $j$th equivariant node to $\sigma(j)$th equivariant node whenever there are both types or only equivariant nodes are existed.
    %     Now, we can similarly define the extended mapping $\Sigma$ between the weight space $\Theta$. 
    %     The edge weight $\Delta \ovt(a, b)$ between the node $a$ and $b$ in $\Delta \ovt$ equals to the edge weight $  \Sigma(\Delta \ovt)(\Sigma(a),\Sigma(b))$ between the node $\Sigma(a)$ and $\Sigma(b)$ in $ \Sigma(\Delta \ovt) $.} 

        Under the helps of the new definitions, we can prove the following lemma.

        \begin{lemma} \label{thm:lemmaGpi}
            For any $\Sigma \in (S_{M} \times S_{N}) $ and $\ovt \in \ovT$,  $ \Sigma(G(s; \ovt))  = G_{}(\Sigma(s);\Sigma(\ovt))$.  
      
        \begin{proof} [(Proof of Lemma)]
        First, we focus on the $l$th neural network layer $\phi(s; \overline{\theta^{l}})$ satisfy that   
      \begin{align} \label{eq:perm_layer}
      \Sigma(\phi(s; \overline{\theta^{l}}))  = \phi(\Sigma(s); \Sigma(\overline{\theta^{l}})). 
    \end{align}
            This property can be derived directly
            from the definition in  \eqref{eq:extensionwb}. 
                %  \begin{equation} \label{eq:sum-kth node}
    %  \rho(\sum_{i=1}^{N} \theta(x_{i},\xi_{x}^{1,x}) ) + \sum_{j=1}^{M} \theta(y_{j},\xi_{x}^{1,x}) +\theta(b_{k}) ) 
    % \end{equation}
    %      where $\rho$ is the non-linear activation function. In the same way, 
    %       the value  for $\Sigma(k)$th invariant node $h_{\Sigma(k)}^{1,x}$ in the layer of $G_{\Sigma(\theta)}^{1}(\Sigma(\bx,\by))$ equals to 
    %      \begin{equation} 
    %       \label{eq:sum-pikth node}
    %         \rho(\sum_{i=1}^{N} \Sigma(\theta)(\Sigma(x_{i}),\Sigma(\xi_{x}^{1,x})) ) + \sum_{j=1}^{M} \Sigma(\theta)(\Sigma(y_{j}),\Sigma(\xi_{x}^{1,x})) +\Sigma(\theta)(\Sigma(b_{k})).
    %      \end{equation}
    %     Recall that we already extended the definition as $\Sigma(\theta)( \Sigma(x_{i}), \Sigma(\xi_{x}^{1,x}) ) = \theta(x_{i}, \xi_{x}^{1,x})$.
    %      Compare the equation (\ref{eq:sum-kth node}) and (\ref{eq:sum-pikth node}) again with the assumption all the activation functions are identical, we can see the values for $\xi_{x}^{1,x} $ in $G_{\theta}$ equals to the value for $h_{\Sigma(k)}^{1,x}$ in  $G_{\Sigma(\theta)}$.
    Furthermore, the neural network $G(s;\ovt)$ simply the repeated composition of the layers $\phi(s;\overline{\theta^{l}})$  with \eqref{eq:perm_layer}. 
    Therefore,  $ \Sigma(G(s; \ovt))  = G(\Sigma(s);\Sigma(\ovt))$.  
    % Therefore, 
    %     $$ \Sigma(\phi^{1}_{{\theta} }(\bx,\by))  = \phi^{1}_{\Sigma(\theta)}(\Sigma(\bx, \by)).$$
    %     It can similarly be shown that 
    %     $
    %     \Sigma(\phi^{2}_{{\theta} }(\bx,\by))  = \phi^{2}_{\Sigma(\theta)}(\Sigma(\bx, \by)) $ and 
    %     $ 
    %     \Sigma(\phi^{3}_{{\theta} }(\by))  = \phi^{3}_{\Sigma(\theta)}(\sigma '( \by)).
    %      $
    %     Finally,  $ \Sigma(G_{{\theta} }(\bx,\by))  = G_{\Sigma(\theta)}(\Sigma(\bx, \by)) $ can be established by function coposition of $\phi_{\theta}^{i}$ and $\phi_{\Sigma(\theta)}^{i}$. 

        \end{proof}
    \end{lemma}
Now, we are able to show 
$
  % \label{eq:LpiveqLv}
  l_{G}(s;\overline{\theta}^{*}+\Delta \ovt) = l_{G}(s;\overline{\theta}^{*}+\Sigma(\Delta \ovt)) $ for any $\Sigma$,  $\Delta \ovt$, and  $\overline{\theta}^{*}$. 
  From the definition of the loss function $l_{G}$ in the equation (\ref{eq:loss}), for any $\Sigma_{0} \in S_{N} \times S_{M}$, 
  \begin{equation*}
    \begin{split}
      l_{G}(s;\overline{\theta}^{*}+\Sigma(\Delta \ovt)) & = \sum_{\Sigma \in (S_{N}\times S_{M}) } \vert Q_{\pi^{\star}}(\Sigma_{0} \circ \Sigma(s)) - G (\Sigma_{0} \circ \Sigma(s);\ovt^{*}+ \Sigma_{0}(\Delta \ovt))  \vert ^{2}  \\ 
      & =  \sum_{\Sigma \in (S_{N}\times S_{M}) } \vert  Q_{\pi^{\star}}(\Sigma_{0} \circ \Sigma(s)) -  G (\Sigma_{0} \circ \Sigma(s);\Sigma_{0}(\ovt^{*}+\Delta \ovt))  \vert ^{2}  \quad (\because \Sigma_{0}(\ovt) = \ovt) \\
      &  =  \sum_{\Sigma \in (S_{N}\times S_{M}) } \vert \Sigma_{0} (Q_{\pi^{\star}}(\Sigma(s))) - \Sigma_{0} (G (\Sigma(s);\ovt^{*}+\Delta \ovt))  \vert ^{2}   \qquad (\because \text{from Lemma \ref{thm:lemmaGpi}}) \\
    &  =  \sum_{\Sigma \in (S_{N}\times S_{M}) } \vert Q_{\pi^{\star}}(\Sigma(s)) -G  (\Sigma(s);\ovt^{*}+\Delta \ovt) \vert ^{2}  \\
    & =  l_{G}(s; \ovt^{*}+ \Delta \ovt) .
    \end{split}
  \end{equation*}

  Furthermore, the directional derivative $D_{\Sigma(\Delta \ovt)}(L_{\ovt^{*}})$ along $\Sigma(\Delta \ovt)$ would be
  \begin{equation*}
    \begin{split}
      D_{\Sigma(\Delta \ovt)}(l_{G}(s;\ovt^{*})) & = \lim _{h \rightarrow 0} \frac{l_{G}(s;\ovt^{*}+h \Sigma(\Delta \ovt)) - l_{G}(s;\ovt^{*})}{h} =  \lim _{h \rightarrow 0} \frac{l_{G}(s;\ovt^{*}+h \Delta \ovt) - l_{G}(s;\ovt^{*})}{h}  = D_{\Delta \ovt}(l_{G}(s;\ovt^{*}))<0.
    \end{split}
  \end{equation*}
  The existence of the limit is induced from the assumption  about the differentiability of the activation function $\rho$. 
  Furthermore,  
 since the activation function is continuously differentiable, when we define $\Delta \theta \in \ovT$  as the summation of $\Sigma(\Delta \ovt)$ for all $\Sigma$ or $\Delta \theta : = \sum_{\Sigma} \Sigma(\Delta \ovt)$, $$D_{\Delta \theta}(l_{G}(s;\ovt^{*}) ) = \sum_{\Sigma} D_{\Sigma(\Delta \ovt)}(l_{G}(s;\ovt^{*})) < 0. $$

  From the symmetricity of $\Delta \theta$ due to the $\Sigma \in S_{N} \times S_{M}$, 
  there exists a vector  $\theta_{0} \in \Theta $  such that 
    $\Delta \theta =\overline{\theta_{0}}$.
    Thus, $D_{\theta_{0}}(L_{F}(s;\theta^{*})) $ being the negative derivative of the loss function 
    $L_{F}(s;\theta^{*})$ along $\theta_{0}$  contradicts the assumption that $\overline{\theta}^{*}$ is the local minima on the loss surface $L_{F}(s;\theta^{*})$.  

  \end{proof}

  \subsection{Proof of Theorem~\ref{thm:universal}} \label{sec:thm_univ}
  \begin{figure}
    \includegraphics[width=0.5\linewidth]{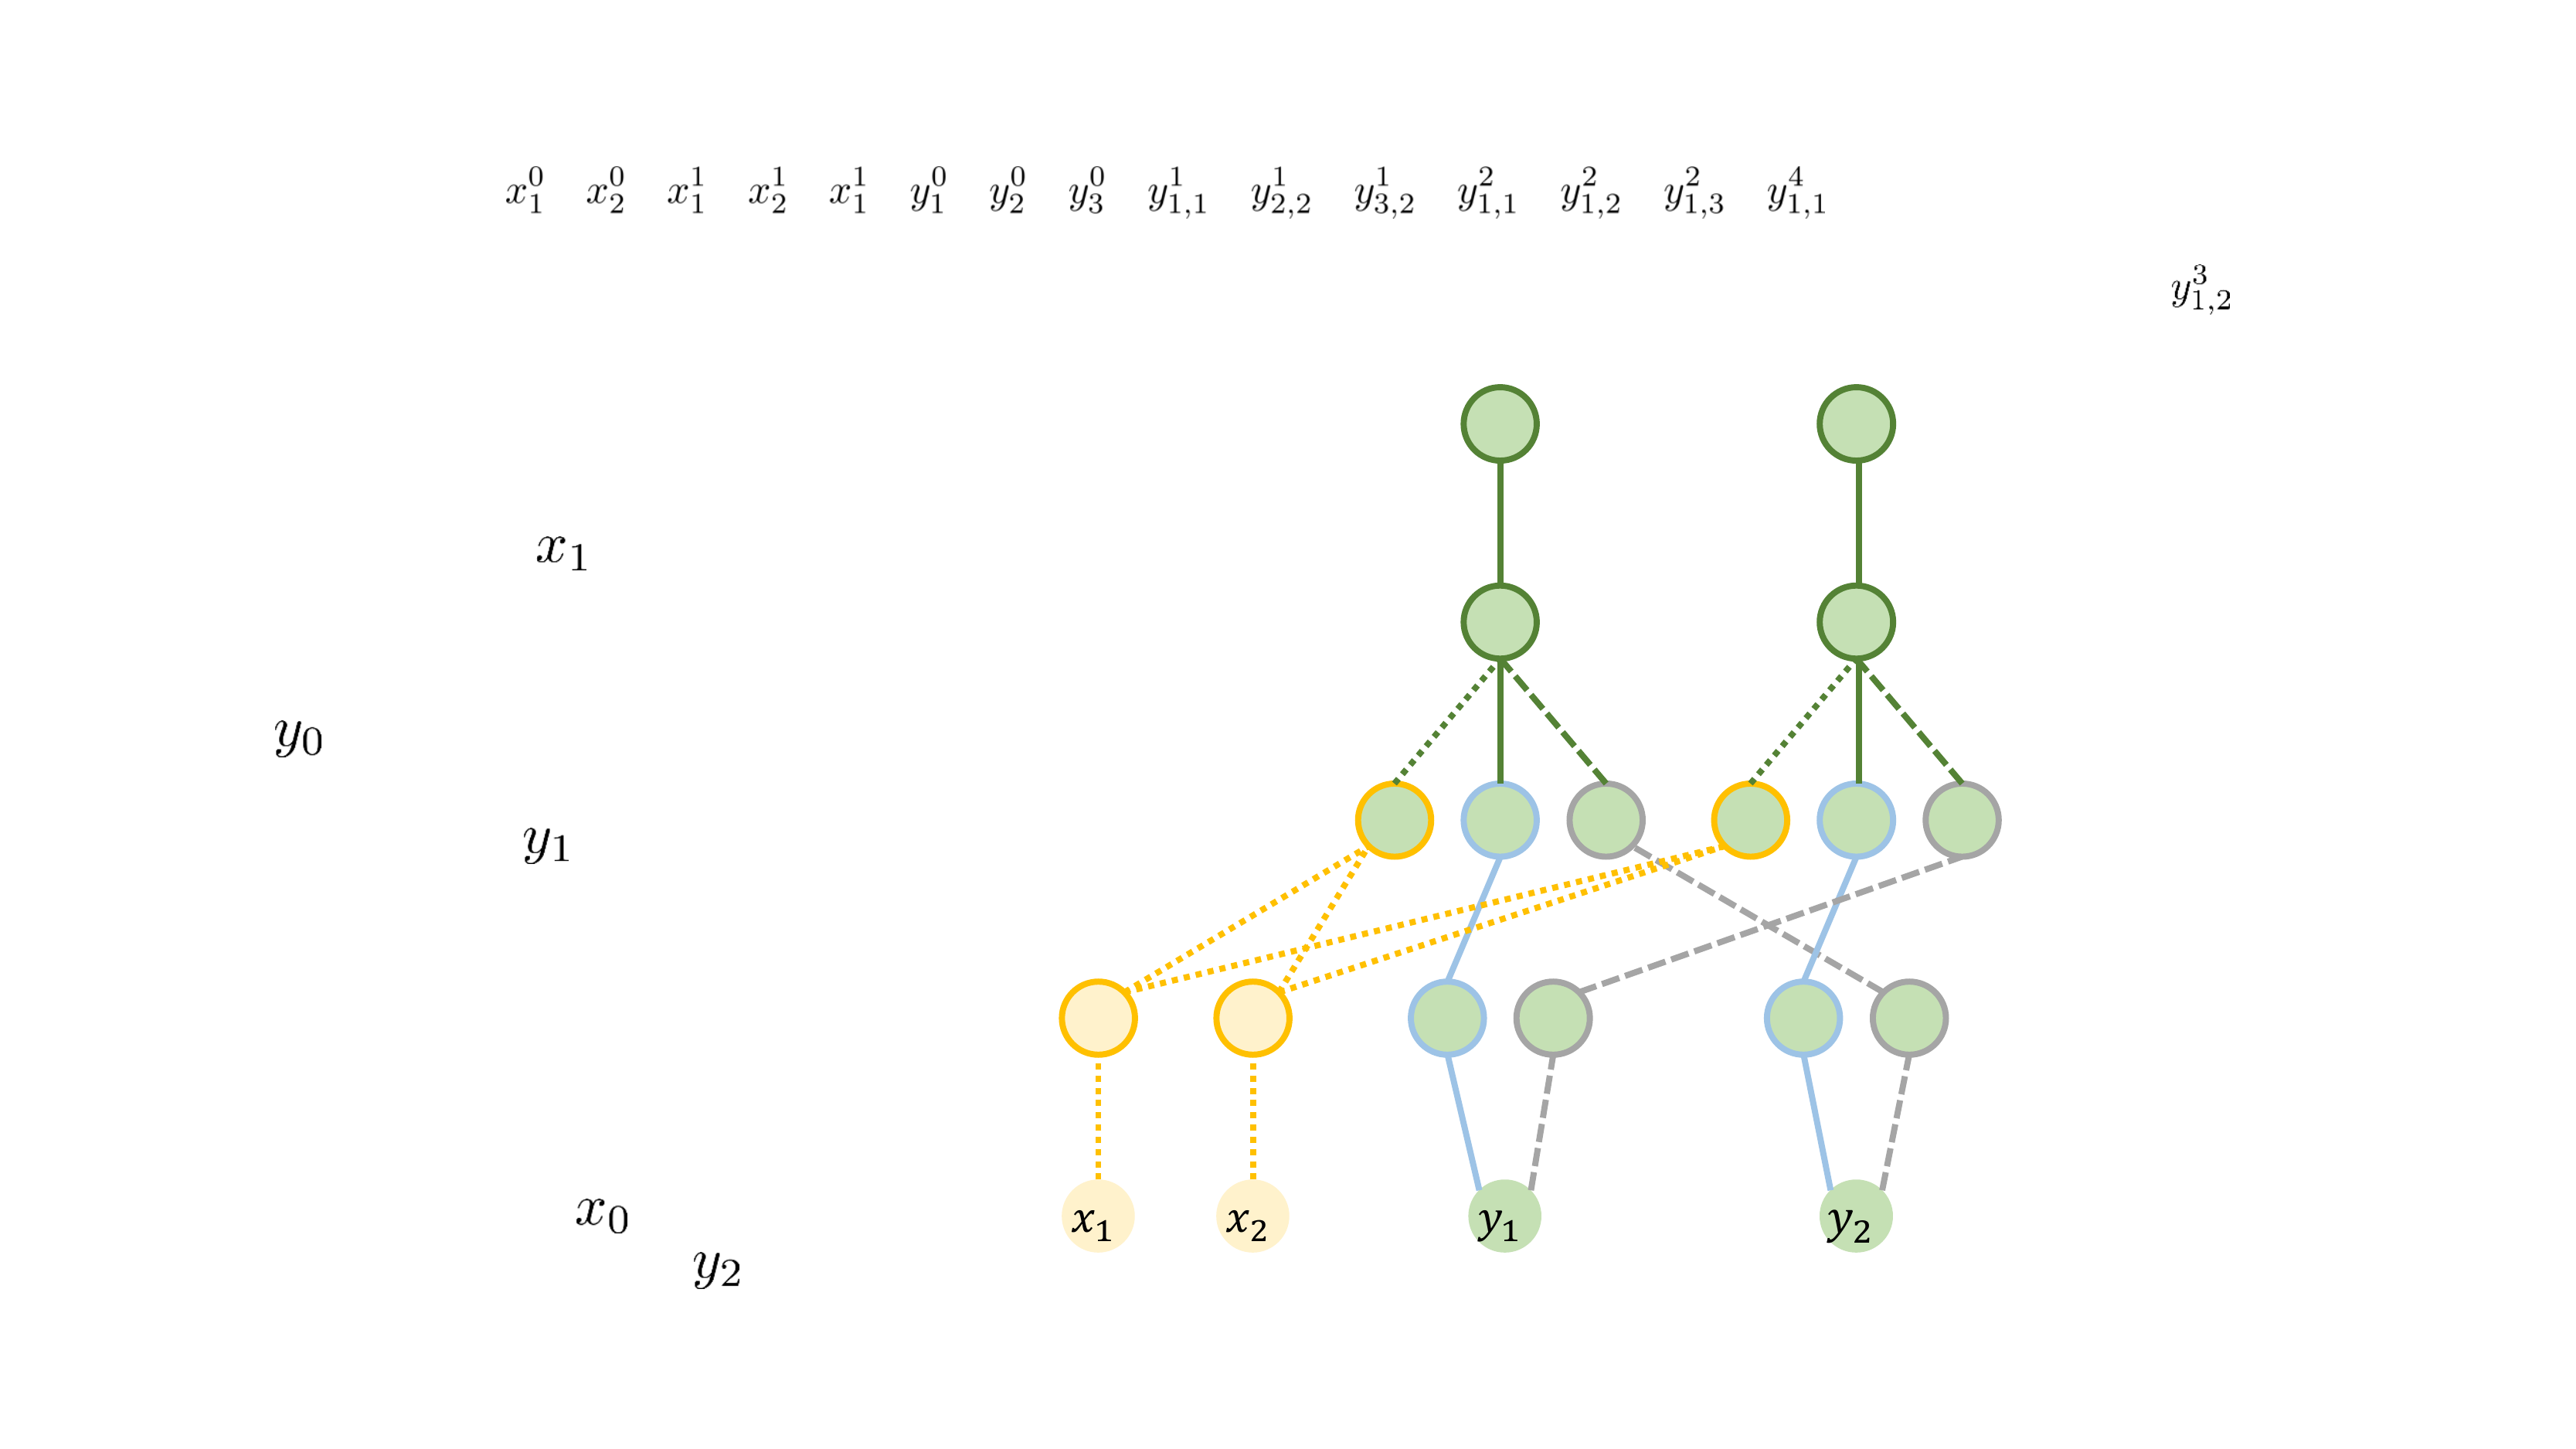}
    \centering 
    \caption{A simplified version of intra-shared neural network $Q_{\theta}(\bx,\by)$ when $l=m=2$ to approximate $f(\bx,\by)$. 
    If edges share the same color and shape in the same layer, the corresponding weight parameters are tied together. 
    Each node represents a multiple dimensional vector. 
    The same colored edges represent the functions in Lemma~\ref{thm:universal}: $H, \sum_{x \in \bx} \xi_{x}(x), y, \sum_{y \in \by_{-1}} \xi_{y}(y).$
    The apricot colored edges represent a mapping: $y_{1}^{2} = (y_{1,1}^{2}, y_{1,2}^{2}, y_{1,3}^{2}) \rightarrow y_{1,1}^{3} \rightarrow y_{1,1}^{4}$ is an approximation of $H(\sum_{x \in \bx} \xi_{x}(x), y_{1}, \sum_{y \in \by_{-1}} \xi_{y}(y))$. 
    The yellow dotted lines represent a mapping: $x_{1}^{0} \rightarrow x_{1}^{1} \rightarrow y_{1,1}^{2}$ represent the function $\xi_{x}(x)$. 
    The sky blued solid lines represent an identity mapping: $y^{0}_{1} \rightarrow y_{1,1}^{1} \rightarrow y_{1,2}^{2}$ for $y_{1}$ in $H$.
    Finally, the grey dashed lines represent $\xi_{y}(y)$. 
    % The 3 nodes $y^{2}_{1,1}, y^{2}_{1,2},y^{2}_{1,3}$ have roles of the inputs of the function $H(\sum_{x \in \bx} h_{x}(x),h_{1}(y_{1}), \sum_{y \in \by_{-i}}\xi_{y}(y))$ respectively. 
    }  
    \label{fig:universe}
    \end{figure}
\begin{proof}
Let $[f(\bx,\by)]_{p}$ as the $p$th row of output of $f(\bx,\by):\cX^{l} \otimes \cY^{m} \rightarrow \Real^{m} \otimes \Real^{\vert \cC \vert}$, i.e.,  
$$ f(\bx,\by)=([f(\bx,\by)]_{1},\cdots, [f(\bx,\by)]_{m}). $$
It is enough to check that a function $[f(\bx,\by)]_{p}: \cX^{l} \otimes \cY^{m} \rightarrow \Real ^{\vert \cC \vert}$ can be approximated by the $p$th row $[Q_{\theta}(\bx,\by)]_{p}$ of the I-shared neural network $Q_{\theta}(\bx,\by)$.
Without loss of generality, we focus on the case  when $p=1$.  
% since the both $Q_{\theta}$ and $f(\bx,\by)$ have the permutation equi-invariant property.   
  From the equi-invariance of $f(\bx,\by)$, $[f(\bx,\by)]_{1}: \cX ^{l} \otimes \cY \otimes \cY^{m-1} \rightarrow \Real ^{\vert \cC \vert}$ 
  is permutation invariant to the orders of $\bx=(x_{1}, \cdots, x_{l})$,  $(y_{1})$, and $\by_{-1}:=(y_{2}, \cdots, y_{m})$, i.e., 
  \begin{equation}
   \forall \sigma_{l} \in \bS_{l}, \text{ } \forall \sigma_{m-1} \in \bS_{m-1}, \quad [f(\bx,y, \by_{-1})]_{1} \equiv [f(\sigma_{l}(\bx), y, \sigma_{m-1}(\by_{-1}))]_{1}. 
  \end{equation} 
  In Lemma~\ref{thm:lem_conti_repr}, we derive that any continuous function with the above symmetry can be decomposed in the form of $ H(\sum_{x \in \bx} \xi_{x}(x), y_{1}, \sum_{y \in \by_{-1}}\xi_{y}(y))$ where $H, \xi_{x}, \xi_{y}$ are proper continuous functions. 
  Finally, we will show that $Q_{\theta}$ with more than 4 layers can approximate the decomposed form of $[f(\bx,\by)]_{1}$. 
  % For notational convenience, we will abuse some notations $\xi_{x}(\bx):=\sum_{x \in \bx} \xi_{x}(x)$ and $\xi_{y}(\by_{-1}):=\sum_{y \in \by_{-1}}\xi_{y}(y)$. 
\begin{lemma} \label{thm:lem_conti_repr}
  Suppose a continuous function $F(\bx,\by, \bz):\cX^{l} \otimes \cY^{m} \otimes \cZ^{o} \rightarrow \Real^{d}$ is defined on a compact space with $l,m,o \in \naturalint$. 
  The function $F$ is permutation invariant to the orders of the items in $\bx \in \cX^{l}, \by \in \cY^{m}, \bz \in \cZ^{o}$, i.e., 
  $$ \forall \sigma_{l} \in \bS^{l}, \text{ }\forall \sigma_{m} \in \bS^{m}, \text{ }\forall \sigma_{o} \in \bS^{o}, \quad F(\sigma_{l}(\bx), \sigma_{m}(\by), \sigma_{o}(\bz)) \equiv F(\bx,\by,\bz).  $$
  if and only if $F(\bx,\by,\bz)$ can be represented by proper continous functions  $H, \xi_{x}, \xi_{y}$,and $\xi_{z}$ with the decomposed form of 
  \begin{equation} \label{eq:Hxyz}
  F(\bx,\by,\bz)= H(\sum_{x \in \bx}\xi_{x}(x), \sum_{y \in \by}\xi_{y}(y),  \sum_{z \in \bz}\xi_{z}(z)).
  \end{equation}
  \begin{proof} 
  (Sufficiency) The sufficiency is easily derived from the fact that $\sum_{x \in \bx}\xi_{x}(x), \sum_{y \in \by}\xi_{y}(y)$, and $  \sum_{z \in \bz}\xi_{z}(z)$ are permutation invariant to the orders of $\bx, \by, \bz$ respectively.
  Therefore,  $H(\sum_{x \in \bx}\xi_{x}(x), \sum_{y \in \by}\xi_{y}(y), \sum_{z \in \bz}\xi_{z}(z))$ is permutation invariant to $\bx,\by,\bz$.  
  
  % \begin{equation*}
  %   \begin{split}
  %    \exists \xi_{x}, g_{k} \in C(\Real),\forall \bx \in [0,1]^{k}, \quad   g_{k}(\sum_{x \in \bx} \xi_{x}(x)) = \bx, \\ 
  %    \exists \xi_{y}, \xi_{y} \in C(\Real),\forall \by \in [0,1]^{m}, \quad   \xi_{y}(\sum_{y \in \by} \xi_{y}(y)) = \by, \\ 
  %    \exists \eta_{z}, \xi_{z} \in C(\Real),\forall \bz \in [0,1]^{l}, \quad   \xi_{z}(\sum_{z \in \bz} \eta_{z}(z)) = \bz.
  %   \end{split}
  % \end{equation*}
  (Necessity) 
  % Without loss of generality, we assume that $\cX=\cY=\cZ = [0,1]$.
  Without loss of generality, we assume that $\cX = \cY = \cZ = [0,1]$. 
  Our lemma follows a result of Theorem 7 in \cite{zaheer2017deep} about the existences of 6 continuous functions described below.
  \begin{equation}
  \begin{array}{llr}
     \exists \eta_{x} \in C([0,1]^{l+1}, [0,1]^{l}), & \exists \xi_{x} \in C([0,1],[0,1]^{l+1}), & \eta_{x}(\sum_{x \in \bx} \xi_{x}(x)) := \bx, \\  \exists \eta_{y} \in  C([0,1]^{m+1}, [0,1]^{m}), & \exists \xi_{y} \in C([0,1], [0,1]^{m+1}),  & \eta_{y}(\sum_{y \in \by} \xi_{y}(y)) := \by, \\   \exists \eta_{z} \in C([0,1]^{o+1}, [0,1]^{o}), & \exists \xi_{z} \in C([0,1], [0,1]^{o+1 }), & \eta_{z}(\sum_{z \in \bz} \xi_{z}(z)) := \bz. 
  \end{array}
  \end{equation}
  Therefore, we can define a continuous function $H(\cdot,\cdot,\cdot): \Real^{l+1} \otimes \Real^{m+1} \otimes \Real^{o+1} \rightarrow \Real^{d}$ as 
   $$H(\cdot,\cdot,\cdot):= F(\eta_{x}(\cdot), \eta_{y}(\cdot), \eta_{z}(\cdot)).$$
   It is obvious that the function $H$ satisfies \eqref{eq:Hxyz}. 
  \end{proof}
\end{lemma}
With the result of the lemma, the only remained problem to check is that $Q_{\theta}(\bx,y_{1}, \by_{-1})$ with more than 4 layers is able to approximate $H(\sum_{x \in \bx} \xi_{x}(x), y_{1}, \sum_{y \in \by_{-1}}\xi_{y}(y))$. 
Before a detailed explanation, we set some notations of the nodes in $Q_{\theta}$.  
Recall Section~\ref{sec:IntraSharing}, the $h$th layer of $Q_{\theta}(\bx,\by)$ is represented as $(\bx^{h},\by^{h})$ where $\bx^{h}:=(x^{h}_{1}, \cdots, x^{h}_{l})$  and  $\by^{h}:=(y^{h}_{1}, \cdots, y^{h}_{m})$ are relevant to the orders of $\bx, \by$ respectively except the final layer $[Q_{\theta}(\bx,\by)]_{4}$.  
% Automatically, the input layer $(\bx^{0},\by^{0})=(\bx,\by)$ and the first node vector $y_{1}^{4}= [Q_{\theta}(\bx,\by)]_{1}$. 
The nodes in $\bx^{h}$ or $\by^{h}$ can be multiple dimensional vectors since $Q_{\theta}$ is able to have multiple channels. 
We sometimes handle a node vector as an tuple of multiple node vectors. 
An simplified version of $Q_{\theta}$ is described in Figure~\ref{fig:universe}.
In the figure, we use $(y_{j,1}^{2}, y_{j,2}^{2}, y_{j,3}^{2})$ to represent 3 components of $y_{j}^{2}$, i.e., for $j=1$ or $2$, $y_{j}^{2}=(y_{j,1}^{2}, y_{j,2}^{2}, y_{j,3}^{2})$.  
Finally, let $ W_{\theta}(node_{1}, node_{2}): \Real^{dim(node_{1})} \rightarrow \Real^{dim(node_{2})} $ denote an mapping from $node_{1}$ to $node_{2}$ including a weight matrix and a bias in $Q_{\theta}$.

We shall show 
the existence of a proper set of the weight parameters $\theta$ 
that the components $\sum_{x \in \bx}\xi_{x}(x)$,  $\sum_{y \in \by_{-1}}\xi_{y}(y)$, $y_{1}$, and $H$ can be approximated without violating the intra-sharing rule. 
We exploit the universal approximation theorem in \cite{gybenko1989approximation} which shows that any continuous function $f$ 
on a compact domain can be approximated by a proper 2-layered neural network $f_{\omega}$ satisfied $\Vert f-f_{\omega} \Vert_{\infty} <\epsilon$ for any $\epsilon>0$. 
% For all $(i,j) \in \{1,\cdots, k\} \times \{1,\cdots, N-k\}$, 
For any $(i,j,r) \in \{ (i,j,r) \vert 1 \leq i \leq l, 1 \leq j,r \leq m, j \neq r\}$, 
we set $W_{\theta}(x_{i}^{0},x_{i}^{1})=W_{2}$ and $W_{\theta}(x_{i}^{1},y_{j,1}^{2})=W_{1}$ where $W_{1}$ and $W_{2}$ are the mappings that satisfy $W_{1} \circ W_{2} (x) \approx \xi_{x}(x)$.
It is easily achieved that the node vector $y_{j,1}^{2}$ satisifies the below statement. 
 $$y_{j,1}^{2} = \sum_{x \in \bx} W_{2} \circ W_{1} (x)  \approx \sum_{x \in \bx}\xi_{x}(x) \quad \text{ (yellow dotted lines)}.$$ 
In the similar way, there exist proper mappings $W_{3}$, $W_{4}$ which approximates $W_{3} \circ W_{4}(y) \approx y$. 
We set $W_{\theta}(y_{j,1}^{1}, y_{j,2}^{2}):= W_{3}$ and $ W_{\theta}(y_{j}^{0}, y_{j,1}^{1})=W_{4}$ follows the intra-sharing rule. 
Therefore, $$ y_{j}^{2} =  W_{\theta}(y_{j,1}^{1}, y_{j,2}^{2}) \circ  W_{\theta}(y_{j}^{0}, y_{j,1}^{1})(y_{j}) =  W_{3} \circ W_{4}(y_{j}) \approx y_{j} \quad \text{ (blue solid lines)}. $$ 
Let $W_{\theta}(y_{j,1}^{1},y_{r,2}^{2}):= W_{5}$ and $ W_{\theta}(y_{j}^{0}, y_{j,2}^{1}):=W_{6}$ with $W_{5} \circ W_{6}(y) \approx \xi_{y}(y)$ so  
$$y_{j,2}^{1} = \sum_{y \in \by_{-j}} W_{\theta}(y_{j,1}^{1},y_{r,2}^{2}) \circ W_{\theta}(y_{j}^{0}(y) , y_{j,2}^{1})(y) \approx \sum_{y \in \by_{-j}} \xi_{y}(y) \quad \text{ (grey dashed lines)}.$$ 
Finally, we can also find a 2-layered mapping $(y_{j,1}^{2}, y_{j,2}^{2}, y_{j,3}^{2}) \rightarrow y_{j,1}^{3} \rightarrow y_{j,1}^{4}$ which is an approximation of $H(\cdot, \cdot, \cdot)$.  
To sum up, the 1st row of the overall neural network $$[Q_{\theta}(\bx,\by)]_{1} \approx H(\sum_{x \in \bx} \xi_{x}(x), y_{1}, \sum_{y \in \by_{-1}}\xi_{y}(y))=[f(\bx,\by)]_{1}. $$ 
\end{proof}

% \section{Equi-Invariant Property in select-MDP}
% \begin{prop}
% For any arbitrary permutation $\sigma_{N}$ and $\sigma_{K}$, the optimal action-value function $Q^{\star}$ in select-MDP has permutation invariant property 
% $$Q(s,a) =Q(\sigma_{N}(s), \sigma_{N} \circ \sigma_{K}(a)).$$ 
% In greedy select-MDP, $\tQ^{\star}$ satisfies the permutation invariant property with the above permutation $\sigma$ as
% $$\tQ^{\star}(\ts, \ta) = \tQ^{\star}(\sigma_{\ts}(\ts),  \sigma_{\vert \tby \vert}(\ta)). $$
% \end{prop}

\section{Detailed Experiment Settings}  \label{sec:experiment}
In this subsection, we explain the environment settings and algorithm performances in more detail.

\subsection{Evaluation Settings} \label{sec:Evaluation Settings}
\paragraph{Sequential Circle Selection}
As mentioned in Section \ref{sec:SequentialCircle},  The game consists of $N$ selectable and $U$ unselectable circles within a $1 \times 1$ square area, as shown in Figure ~\ref{fig:circles}. Here, circles are the items and $i_{n} :=(pos_x, pos_y, radius)$ are their contexts, where $pos_x$ and $pos_y$ are their center coordinates. There is a single command which is to select the circle. Initially, all circles have random coordinates and radius, sampled from $U(-0.6, 0.6)$ and $U(0, 0.4)$, respectively, where $U$ is random uniform distribution. Each time the agent finishes choosing $K$ circles, transition occurs as follows. Selected circles disappear. Unselectable circles that collide with the selected circles disappear. New circles replace the disappeared circles, each of initial radius $0.01$ and random coordinates sampled from $U(-0.6, 0.6)$. Remaining circles expand by $0.05$ in radius (maximum radius $0.4$) and move with a noise sampled from $U(0, 0.1)$. The agent also receives reward $R$ after the $K$th selection, calculated for each selected circle $k$ of area $A_{k}$ as follows: \textit{Case 1.} The selected circle collides with one or more unselectable circle: $R = -A_{k}$. \textit{Case 2.} Not case 1, but the selected circle collides with another selected circle: $R = 0$. \textit{Case 3.} Neither case 1 nor 2: $R = A_{k}$. We experimented with two different numbers of elements to select: $K=1$ and $K=3$.

\subsection{Predator-Prey}

\subsection{Multi-type EINET}
Our environments contain unselectable items as well as selectable items. Such multi-type element setting is a common and scenario in many real applications. Note that additional permutation invariance applies to the unselectable items. Correspondingly, the EINET in our experiment has three input types: equivariant inputs, invariant inputs for selected items, and invariant inputs for unselectable items.

\subsection{Hyperparameters}
\label{sec:hyperparameters}
\begin{table}[h]
  \small
  \centering
  \caption{Training hyperparameters}
  \label{table:hyperparam}
  \begin{tabular}{L{4.5cm}L{1.2cm}L{7cm}}
    \bf{Hyperparameter} & \bf{Value} & \bf{Description} \\ \midrule
    Buffer size & 50,000 & Size of replay buffer used to store transitions \\
    Minibatch size & 128 & Number of transitions sampled from replay buffer in each step \\
    Learning rate & 0.003 & Learning rate used by Adam optimizer \\
    Discount factor & 0.99 & Discount factor $\gamma$ used in Q-learning update \\
    Target network update frequency & 200 & The frequency (measured in number of training steps) 
    with which the target network is updated \\
    Initial exploration & 1 & Initial value of $\epsilon$ used in $\epsilon$-greedy exploration \\
    Final exploration & 0.05 & Final value of $\epsilon$ used in $\epsilon$-greedy exploration \\
  \end{tabular}
\end{table}

\subsection{Evaluation}
random seeds, how the reward is measured (averaged) \note{TODO}

\subsection{Performance Analysis} \label{sec:Performance Analysis}
Our EINET outperforms other baselines, particularly as $N$ grows large. We briefly discuss the reasons by introducing our intuitions for the problems of the baselines.  

% \paragraph{Shuffling} By using permuted examples during training, this method helps the agent experience various orders of elements, making the agent naturally learn the symmetry. It also has an additional effect of preventing correlation between states and overfitting of the policy. Nevertheless, when the number of homogeneous elements is very large, the agent may not be able to learn all the equivalent experiences during training. Thus, the drawback of this method is that it is computationally intractable for large $N$. \note{check}

\myparagraph{Sorting} Sorting is depends on a specified rule to choose a representative among all the equivalent states. However, different rules result in different training procedures, which create different agents. A more serious pitfall of sorting is that it can neglect the almost-equivalence of two almost states and regard them as two totally different states. For example, consider the states composed of two homogeneous equivariant elements: $\{(1,1), (8,0.99) \}$ and $\{ (1,0.99), (8,1) \}$. In EINET, they are treated as almost the same, since their values are similar. In sorting, however, if the agent sorts the states by $y$ values in descending order, the two states become $\{(1,1), (8,0.99) \}$ and $\{(8,1), (1,0.99) \}$, which would be regarded as different states by the agent. 
% \note{check}

\myparagraph{Rule-based heuristics} The design of the rule-based heuristics is as follows. As a primary choice, either choose the largest isolated selectable circle or destroy a big ($r>0.2$) unselectable circle by choosing the smallest selectable circle that collides with it. If primary choices are no more available but still $k<K$,  select the smallest selectable circle in the environment that satisfies the two conditions. First, it should be smaller than the largest previously chosen isolated circle. Second, it should not collide with any previously chosen isolated circle. If even secondary choices run out (which is an extremely rare case) choose a random selectable circle. Figure ~\ref{fig:greedy_fail} shows two scenarios where the heuristics fails to achieve petter performance.

\begin{figure*}
  \centering
  \subfloat[Figure 1]{\label{fig:1}\includegraphics[width=0.49\textwidth]{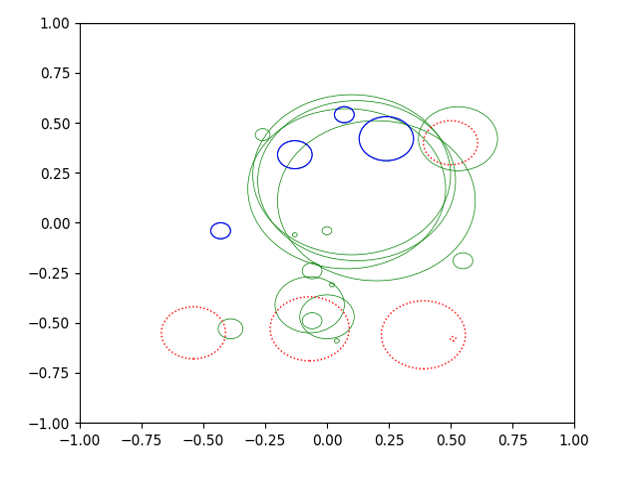}}
  \subfloat[Figure 2]{\label{fig:2}\includegraphics[width=0.49\textwidth]{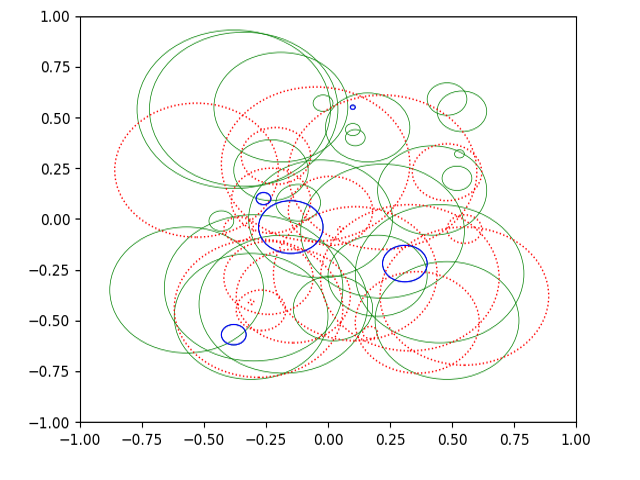}}
  % \begin{subfigure}[t]{0.5\textwidth}
  %   \centering
  %       \includegraphics[width=0.49\textwidth]{figure/greedy_fail_1}
  %       \caption{blua}
  %       \label{fig:1}
  % \end{subfigure}
  %     \subfloat[\small trio capture]{\label{fig:2}
  %       \includegraphics[width=0.49\textwidth]{figure/greedy_fail_2}}
  % \end{center}
  % \vspace{-0.6cm}
  \caption{Scenarios when heuristics perform worse than EINET. Blue circles are selected, green circles are other selectable circles, red circles are unselectable circles. \ref{fig:1} Considering long-term effects. Better to first remove the unselectable circle on the top right, even if this would result in smaller reward at current step. \ref{fig:2} Considering joint effects. Unnecessary selection of four circles, since they have overlapping effects.}
  \label{fig:greedy_fail}
  \end{figure*}
\end{appendices}
